# Supplementary material for: Dissertation Paths: Advisors and Students in the Economics Research Production Function
Source: arXiv:2501.01533 ancillary file (2025-02-17)
Supplement: Supplementary file 1 [file DissePathsAppendix021725.pdf]

# Appendix to “Dissertation Paths: Advisors and Students in the Economics Research Production Function”

Joshua Angrist\*   Marc Diederichs<sup>†</sup>

with

Alison Fang   Merilin Martinson   Isabel Munoz   Margaret Zheng

December 2024

---

\*MIT and NBER. Email: [angrist@mit.edu](mailto:angrist@mit.edu)

<sup>†</sup>ROCKWOOL Foundation Berlin and University of Passau. Email: [md@rfberlin.com](mailto:md@rfberlin.com)

# Contents

|          |                                                                        |           |
|----------|------------------------------------------------------------------------|-----------|
| <b>1</b> | <b>Data Set Construction</b>                                           | <b>1</b>  |
| 1.1      | Student and Advisor Data Sources . . . . .                             | 1         |
| 1.2      | Merging Sources . . . . .                                              | 3         |
| 1.3      | Student Department Classification . . . . .                            | 3         |
| 1.4      | Analysis Samples . . . . .                                             | 4         |
| 1.5      | Identifying Advisors: Details . . . . .                                | 4         |
| 1.6      | Measuring Productivity . . . . .                                       | 5         |
| 1.7      | Gender and Affinity Measures . . . . .                                 | 6         |
| 1.8      | GPT Enhancements to Advisor Identification Using Thesis PDFs . . . . . | 7         |
| <b>2</b> | <b>Publications Data and Journal Lists</b>                             | <b>9</b>  |
|          | <b>References</b>                                                      | <b>14</b> |

# 1 Data Set Construction

Our goal is to identify all economics PhD graduates who earned economics doctorates between 1989 and 2023 from the following institutions: University of California, Berkeley; University of Chicago; Harvard University; Massachusetts Institute of Technology; Northwestern University; Princeton University; Stanford University; and Yale University. We combine data from five sources to capture the full universe of graduates from these schools. In addition to degree recipients from economics departments, our sample includes degree earners from related programs, such as business and policy schools.

## 1.1 Student and Advisor Data Sources

*ProQuest:* Most US-based PhD students submit their dissertations for publication and archiving through ProQuest’s ETD Administrator web site. ProQuest, publisher of the *Web of Science* database of journal articles, also publishes the *Dissertations and Theses* database (formerly *Dissertation Abstracts*). A student’s graduate school reviews the submission before ProQuest finalizes the publication and archival process. Student submitters choose a research field, which ProQuest stores in the `classterm` variable. Our initial sample includes approximately 9,330 ProQuest students with `classterm`="economics". According to the 2022-2023 ProQuest Subject Categories list, students are asked to choose one category that “best describes [their] field of research of creative work” and may add 1-2 additional categories that “will also be associated with [their] work as secondary subjects”. In practice, some people list up to 5 classifications.

We access ProQuest data via the ProQuest TDM Studio online interface, using Python scripts to compile a dataset that includes student names, degree years, schools, titles, advisors, and dissertation committee members. ProQuest data on Ph.D. advisors and committee members are incomplete, however, so we supplement ProQuest with data from additional sources detailed below. Our dataset includes dissertations approved through June 2023.

ProQuest TDM Studio provides metadata about each thesis archived in the ProQuest Dissertations and Theses database, including, in many cases, advisor or thesis committee member names. We supplement this with PDF copies of full dissertation texts obtained through the ProQuest interface accessed via university libraries, where available. Thesis PDFs are searched for information not included in the TDM Studio metadata. Specifically, we use PDFs to add department affiliation, advisor names, and research affinity variables like student citations to their advisors. PDF processing is described below.

TDM studio provides a unique dissertation identifier that we use to link to PDFs. For students whose metadata were obtained outside of TDM Studio, however (e.g., from Econlit), we search for PDFs using student name, approximate graduation year, and degree-granting institution.

*EconLit:* ProQuest omits students who opt to withhold dissertation information. To capture students missing from the ProQuest database and to obtain further information on dissertation topics, we use data from the Journal of Economic Literature (JEL), accessed via EconLit. Each December issue of the JEL lists economics doctorates awarded by U.S. and Canadian institutions for the previous academic year. We obtained JEL data from EconLit, the AEA’s online bibliographic database. The JEL graduate list includes each graduate’s name, degree-granting institution and year, dissertation title, and a JEL subject code for the thesis. Economics or other department staff typically submit degree lists to the JEL; submissions that are too late for the print edition nevertheless appear in Econlit. With about 6,000 graduates, EconLit provides our second most comprehensive list of economics PhD graduates after ProQuest. EconLit data adds around 120 students to the ProQuest graduate list.

*Administrative Records:* Additional information on dissertation advisors and degree-granting departments, as well as a few graduates not found elsewhere, come from administrative records from six economics departments. Departments at Berkeley, Chicago, Harvard, MIT, Northwestern, and Yale provided approximately 3,300 records for their graduates (Princeton and Stanford refused or ignored repeated requests for records). Administrative records typically list graduates’ names, graduation year, and advisor(s) or thesis committee members. Administrative records add roughly 100 additional PhDs, while improving department and advisor information for many others.

*Math Genealogy:* The Math Genealogy project lists PhD recipients for mathematically-oriented disciplines, including economics. Math genealogy (MG) compiles information from individual submissions, ProQuest, and universities. MG aims to link each degree recipient with their PhD students and thesis advisors. We used the MG API to add advisor names for students identified in ProQuest, administrative records, and EconLit. ProQuest might have listed one advisor, say, while MG might include an additional advisor not found elsewhere.

MG includes data on researchers from disciplines other than economics. We therefore limit our attention to the students of advisors who have published in economics journals. Specifically, we start by compiling a list of all economics PhD advisors identified in ProQuest or administrative records who have authored at least three publications listed in EconLit. Section 1.6 details our process for matching advisors from ProQuest or administrative records to their EconLit publications.

Our MG data collection uses the MG API to search for the profiles of the relevant advisors. In the first step, the API search is by first, middle, and last name of an advisor. For advisors without MG profiles sharing these parameters, we search by first and last name only. This generates a list of MG advisors. For each student with at least one MG matched advisor with three or more EconLit publications, we record the student’s name, school, graduation year, MG subject code, and the complete list of their MG advisors. The last step retains PhDs earned between 1989-2023 from one of the eight schools of interest here. The MG sample contributes 31 advisor names for the graduates included in our ProQuest, administrative records, and EconLit sample. For 1992 Berkeley graduate Jushan Bai, for example, MG adds advisor Thomas John Rothenberg.

*DSpace:* DSpace@MIT is a repository for MIT student and faculty research. We used DSpace to add a few economics students graduating from the Sloan School of Management and to add MIT dissertation PDFs.

65 Sloan School PhDs who earned PhDs between 1989-2023 were identified as writing on economics topics and therefore added from DSpace. This list includes, for instance, 2022 graduate Olivia Kim with a thesis on corporate finance advised by Jonathan Parker, Antoinette Schoar, and Joshua Angrist.

MIT thesis PDFs have not routinely been published through ProQuest, though graduating PhD students may now opt in to this. While ProQuest provides metadata for most MIT graduates, including their graduation year and advisors, thesis PDFs are distributed through DSpace@MIT. We search for the DSpace profiles for all MIT economics students who we identified in ProQuest, EconLit, or administrative data. Our search filters for a student’s name and graduation year, downloading dissertation PDFs for each identified student. We retrieved approximately 800 dissertation PDFs for MIT students from DSpace, covering 72 percent of MIT students in our sample. For other schools, we were able to obtain dissertation PDFs for 84 to over 92 percent of students via ProQuest. Even so, we have 2 or 3 advisor names for 85% of MIT students, with one advisor for almost all of the rest (MIT reports advisor names to ProQuest without full PDFs). Across all schools, we downloaded a total of 8241 dissertation PDFs from both DSpace and ProQuest, achieving an overall coverage of 85 percent - though the coverage in the main analysis sample of cohorts 1994-2017 is 93% .

## 1.2 Merging Sources

Data from *ProQuest*, *EconLit*, *department-supplied administrative records*, and *DSpace@MIT* are combined to create our degree recipients database with information on graduates, advisors, and student and advisor research output.

After downloading, cleaning, and formatting the data, sources are merged as follows. We begin with our ProQuest extract, which includes roughly 9,330 students graduating 1989-2023 who classified their thesis as economics. This dataset is merged with approximately 6,000 JEL (Econlit)-listed graduates using student name, graduation year, and school.

The merge resolves discrepancies in graduation years or names due to typos or the presence of a middle or second family name (such as for many Hispanic students) in only one source. Student records with similar names and close graduation years are combined when the thesis title matches or is close. Matches are determined by similarity scores assigned using the Stata `matchit` command. This process merges about 5,700 students from EconLit with ProQuest, with around 120 students added to the overall database.

A similar merge adds roughly 150 students from department-supplied administrative records and 50 students from DSpace@MIT. Although some sources contribute only a few students, all sources except EconLit contribute information on students' advisors or committee members. The final sample includes approximately 9,640 economics students found in all sources. Of these, about 6,764 earned degrees from economics departments and another 1,239 earned degrees from closely related departments or programs. These statistics appear in Appendix Table B1.

## 1.3 Student Department Classification

We aimed to build a database of economics PhD students who graduated from an economics or related department or program and to distinguish, where possible, between them. We begin by classifying each student as earning an economics department degree if they appear in the administrative records provided by six economics departments. Next, we use a Python script to scan the initial pages of each thesis PDF (up to the introduction, or the entire thesis if the introduction is not clearly identifiable) seeking mentions of the degree-awarding department or program.

We have complete dissertation PDFs (from ProQuest or DSpace) for 8,330 1989-2023 graduates. Our department-identification script searches for specific keywords associated with program names or departments in the text. We generate a list of possible department and program names across the 8 schools covered by our study, such as "*Department of Economics*" or "*John F. Kennedy School of Government*". A search for these terms is used to classify students as graduates of economics departments or other departments or programs. The latter group is divided into economics-related and other departments or programs.

Out of a total 9,640 1989-2023 graduates, 6,764 students are classified as having earned degrees from economics departments, either because they were included in the administrative spreadsheets or because their thesis states that they graduated from an economics department, excluding departments with compound names such as Agricultural Economics or Business Economics. The group of "economics-related" department or program graduates includes 1,239 students, yielding a total of 8,003 graduates of departments and programs labeled as "Economics", "Finance," "Management," "Business," "Accounting," "Marketing," or "Operations Research" in their department or program name. The remaining group, labeled "other", includes students whose PhD was granted by a department or program unrelated to economics, such as History or Sociology.

Students whose department is not indicated on the first pages of their thesis, whose thesis was not available for download, or who were not included in the administrative spreadsheets are classified into the "economics + related" category if one of their advisors advised at least one

student from this group. Approximately 1,600 students graduated from unrelated programs such as history, sociology or mathematics. These graduates are excluded from most of our analyses.

## 1.4 Analysis Samples

Most of the analyses in the paper use 1994-2017 graduates, allowing 6 years of post-PhD follow-up for the most recent cohort. Our best efforts notwithstanding, the 1994 start was chosen in view of reduced coverage of graduates from some schools in earlier years.

Appendix Table B1 summarizes the 1989-2023 and 1994-2017 graduate samples.

**Table B1:** Number of Graduates per School

|                              | Economics    |                    |               | Related      |                    |               | Other        |                    |               |
|------------------------------|--------------|--------------------|---------------|--------------|--------------------|---------------|--------------|--------------------|---------------|
|                              | Total<br>(1) | Cohort size<br>(2) | Active<br>(3) | Total<br>(4) | Cohort size<br>(5) | Active<br>(6) | Total<br>(7) | Cohort size<br>(8) | Active<br>(9) |
| Panel A. 1989-2023 Graduates |              |                    |               |              |                    |               |              |                    |               |
| Berkeley                     | 1119         | 32.0               |               | 158          | 4.5                |               | 344          | 9.8                |               |
| Chicago                      | 897          | 25.6               |               | 155          | 4.4                |               | 276          | 7.9                |               |
| Harvard                      | 1139         | 32.5               |               | 169          | 4.8                |               | 406          | 11.6               |               |
| MIT                          | 865          | 24.7               |               | 217          | 6.2                |               | 71           | 2.0                |               |
| Northwestern                 | 675          | 19.3               |               | 75           | 2.1                |               | 82           | 2.3                |               |
| Princeton                    | 650          | 18.6               |               | 39           | 1.1                |               | 117          | 3.3                |               |
| Stanford                     | 759          | 21.7               |               | 325          | 9.3                |               | 258          | 7.4                |               |
| Yale                         | 660          | 18.9               |               | 101          | 2.9                |               | 83           | 2.4                |               |
| All                          | 6764         | 24.2               |               | 1239         | 4.4                |               | 1637         | 5.8                |               |
| Panel B. 1994-2017 Graduates |              |                    |               |              |                    |               |              |                    |               |
| Berkeley                     | 854          | 35.6               | .46           | 103          | 4.3                | .36           | 244          | 10.2               | .09           |
| Chicago                      | 681          | 28.4               | .38           | 105          | 4.4                | .53           | 148          | 6.2                | .17           |
| Harvard                      | 791          | 33.0               | .54           | 91           | 3.8                | .42           | 281          | 11.7               | .31           |
| MIT                          | 631          | 26.3               | .58           | 150          | 6.3                | .31           | 42           | 1.8                | .07           |
| Northwestern                 | 485          | 20.2               | .54           | 54           | 2.3                | .50           | 60           | 2.5                | .17           |
| Princeton                    | 467          | 19.5               | .57           | 27           | 1.1                | .44           | 75           | 3.1                | .2            |
| Stanford                     | 530          | 22.1               | .48           | 216          | 9.0                | .46           | 156          | 6.5                | .19           |
| Yale                         | 454          | 18.9               | .52           | 52           | 2.2                | .29           | 48           | 2.0                | .17           |
| All                          | 4893         | 25.5               | .50           | 798          | 4.2                | .41           | 1054         | 5.5                | .19           |

*Note:* Columns 1, 4, and 7 show the sum of graduates throughout 1989-2023 and 1994-2017 that graduated from economics, related or other programs and wrote a thesis classified as economics. Column 2 indicates the average economics program cohort size while column 5 shows how many students from related programs are added on average in the economics + related sample. Column 8 shows the average cohort size for economics-classified students that graduated from a non-economics-related program. Columns 3, 6, and 9 show the share of active graduates of cohorts 1994-2017, where activity is defined as having at least one publication during the six years after graduation (PhD + 1 to PhD + 6) in a Deep impact outlet.

## 1.5 Identifying Advisors: Details

ProQuest reports at least one advisor name for almost all of the graduates in our sample, but often only one. Most economics PhD students have 3 advisors, though many are advised by fewer or by more. We therefore augmented ProQuest (and DSpace) advising information with administrative data, MG, and Chat-GPT applied to thesis PDFs. We sought to identify up to three PhD advisors, though in a few cases found more.

To supplement ProQuest and DSpace information on advisors, we contacted graduate program administrators and faculty heads at the schools in our study, asking for their records on graduate students and advisors. Although we received records from six of the eight universities, these records predominantly cover recent years and omit some advisors leading to a small number of additional advisor identifications. MG adds another 32 advisor names.

Advisors are frequently named in a thesis acknowledgments section or other introductory material. To harvest this information, we used the GPT-4 API. Specifically, we submitted prompts containing the initial pages and acknowledgments section of each dissertation, and asked GPT-4 to identify and list the advisors in a given dissertation. After refining the prompt (detailed in section 1.8), this approach yielded good information on PhD advisors. This automated process left approximately 1250 students missing advisors; we reviewed these students' dissertations manually.

Some of our sources identify "thesis committee members" rather than advisors. Many thesis PDFs, for instance, list committee members. We identify advisors first when these are named as such, followed by thesis committee members when the former are missing. Specifically, we prioritize sources of advisor names as follows:

1. ProQuest advisors, ProQuest committee members
2. admin spreadsheet advisors
3. GPT advisors
4. manual advisors
5. GPT committee members
6. MG advisors

*Disambiguating Advisors:* Advisor names often vary across and within data sources. For example, Joseph G. Altonji might be named as Joe Altonji, Joseph Altonji, or Joseph Gerard Altonji. Additionally, department-provided spreadsheets sometimes use abbreviations or nicknames. To address these variations, we first calculate similarity scores between the advisor names listed for each student. This links "Katz, Lawrence" in, say, ProQuest with "Katz, Larry" on a spreadsheet.

We also compute similarity scores, using Stata's `matchit` command, for all possible pairs of advisors in a given school (pooling years). We review similar names deciding whether they're the same person. Most of these decisions are straightforward, but some require more extensive research. For example, to distinguish between "Steven Levitsky" and "Steven Levitt," who have similar names but are different individuals, we use Google searches and check thesis PDFs.

## 1.6 Measuring Productivity

The research output of students and advisors is measured by counting articles in EconLit. Our copy of EconLit lists more than one million journal articles in nearly 2000 economic and business outlets, around 300,000 collective volume articles such as the Handbook of Labor Economics, and includes variables indicating author names and affiliations.

We merge students and advisors in our sample to the EconLit author variable based on an author's last names and first name initial. This allows us to include all publications even if the first name is abbreviated. For example, most of James Heckman's publications are listed under "Heckman, James" but some are listed under "Heckman, J". For advisors and students with frequent last names we merge using last name and full first name. Where available, middle names are used to discard incorrectly matched publications. Econlit omits middle names for

some authors, so we treat authors with and without a middle name as the same person if the same affiliation is indicated on their publications within a ten-year window. Lastly, we exclude collective volume articles that appeared under the same title as a journal article by the same author.

A scenario in which distinct individuals are associated with a common publication leads in some cases to implausible research productivity. We identify possible cases of misattribution as instances of name duplicates in our database in different schools and years, graduates with more than three publications prior to graduation, and graduates with many changes to affiliation across publications. Taking initial student placement from university websites and the affiliation variable listed with publications into account, we hand-check these by matching our Econlit publications with information on CVs acquired by searching for the scholars on Google.

## 1.7 Gender and Affinity Measures

*Gender Assignment:* We classify gender using first name frequencies from the US Social Security registry. This method assigns a gender to 93% of students and 95% of advisors in our sample. Our gender classification shows 29% of students and 22% of advisors to be female.

*Coauthoring:* To measure research affinity between students and their advisors, we create a dummy variable indicating whether a student has at least one joint publication with one of their advisors in any EconLit-listed outlet before or during their graduation year. This is implemented by searching for the advisor's name in graduates' publication records.

Student classmate coauthoring is coded for each student by first identifying classmates as the set of students who graduated from the same school within two years of the focal student's graduation year. We then look for these classmates as listed authors of works in the focal student's publication record.

*Citations to Advisors: Title search*

Graduate citations of their advisors' work are recorded by looking for appearances in dissertations of the titles of advisor publications found in Econlit. We open each student's dissertation and search for mentions of those titles. Any appearance is assumed to be a bibliographic reference. The sum of the number of times an advisor's publication titles appear in a thesis gives a citation count for each advisor-student combination. Figures 15 and 16 use an ever cited dummy version of this variable. Figure B1 displays the number of publication titles per title length (in words) in our sample. The red distribution only includes publications that were cited at least in one dissertation.

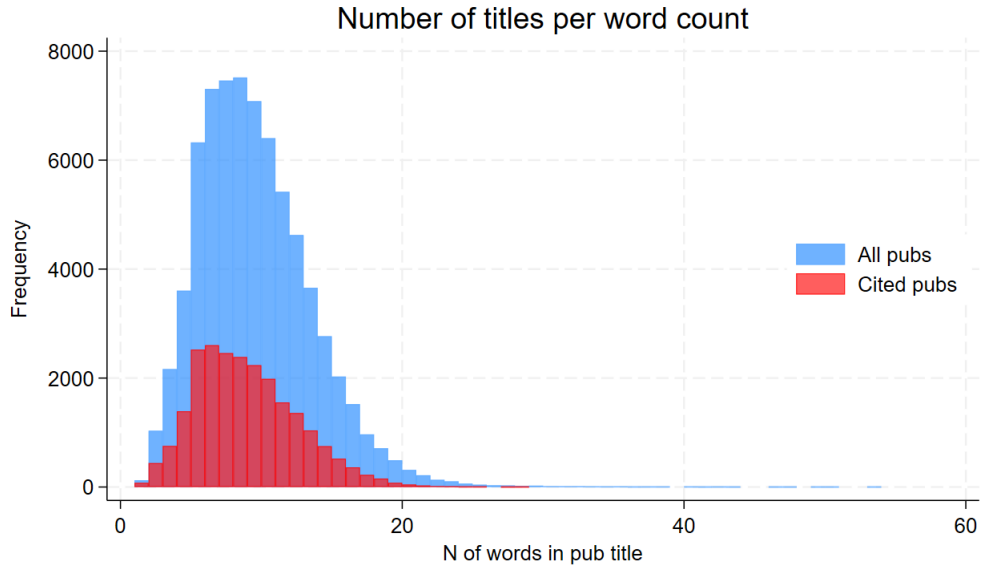

**Figure B1**

This process over-counts short titles (such as *Civil War* or *Regression*) because these words or phrases appear as regular text. We therefore modify title searches to count only those instances of apparent title appearances when the title is enclosed in quotation marks. For dissertations in which bibliographies omit quotation marks, we ignore titles with three words or less when tabulating citation counts.

## 1.8 GPT Enhancements to Advisor Identification Using Thesis PDFs

ProQuest, DSpace, administrative data, and Math Genealogy identify fewer than three advisors for roughly half of graduates. We therefore used ChatGPT to identify advisors in thesis PDFs. This two-step process begins by translating dissertation PDFs into machine-readable text. The text is then part of a prompt submitted to GPT-4. A more detailed and specific prompt reduces false positives (mistakenly-identified advisors) while increasing false negatives (failure to find advisors).

The data used in our prompts consists of the first pages of each dissertation, capped at 3800 tokens. This is typically around 11-12 double-spaced pages or 5-6 single-spaced pages. Below is an extract from the Acknowledgements section of Joshua Angrist's 1989 dissertation from Princeton. Our GPT prompt in this case returns Orley Ashenfelter, David Card, and Whitney Newey as the three advisors. Interestingly, ProQuest identifies Ashenfelter as an advisor while listing Card and Newey as committee members. The Angrist acknowledgement hints at the challenge advisor identification presents: many non-advisor names appear in these two paragraphs, many non-advisors are thanked, and the word advisor does not appear. It's also hard to be sure from this that Angrist's PhD is from the Princeton Department of Economics, which is mentioned only as a source of funding.

In the case of Karyn Model, ProQuest identifies Joshua Angrist as the sole advisor of her dissertation at Harvard. The GPT process correctly finds two more advisors: Richard Freeman and Lawrence Katz.

Special thanks are due to the members my dissertation committee, Orley Ashenfelter, David Card and Whitney Newey. Their contribution to this work cannot be overstated. It was Orley Ashenfelter's keen eye for a

good idea that led me to study the draft lottery. Chapters 1 and 2 benefitted immensely from David Card's careful reading of numerous early drafts and Whitney Newey's private tutoring in econometrics has been invaluable. A partial list of others who made useful comments includes Angus Deaton, Hank Farber, Norman Hearst, Alan Krueger, Kevin Murphy, John Pencavel and Tom Newman.

It is no secret among labor economists that the Industrial Relations Section at Princeton is an exceptional environment for learning and research - it is difficult for me to imagine that there is a better place to work and I will be sorry to leave. Data collection for this project and most of my career as a graduate student were generously funded by the Section. The Section Administrator, Ms. Irene Rowe, who has recently moved on to bigger things, is another important reason my time here has been so pleasant. Thanks also go to the Sloan Foundation for their support of my fourth year of study with a Sloan Foundation Doctoral Fellowship. Financial support of the Princeton Department of Economics and the Olin Foundation is also gratefully acknowledged.

The final template for our prompts appears below. The prompt returns two columns in a Python dataframe, whereby the first is a list of up to three advisor names and the second is a list of any number of committee members for each dissertation. As noted above, for purposes of our analysis, we equate committee members with advisors when there are fewer than 3 of the latter (based on all sources).

```
# Function that connects to openai's API and requests:
## advisors, committee members

## input: first X characters of a dissertation
## output: python code that generates a row for a dataframe

def chatGPT(text):

    # Define OpenAI credentials to connect to ChatGPT

    openai.organization = org
    openai.api_key = key

    input = [
        {"role": "system", "content": "You are a helpful assistant."},
        {"role": "user", "content": text},
        {"role": "user", "content": ""}
    ]
    Act as a researcher reading through dissertation text.
    You will have 2 tasks. Use the same text for all.

    Whenever you cannot find a name for any of the tasks, use instead None.

    Task 1: Find the names of 3 unique PhD dissertation advisors from this
    text.

    Your aim is to find 3 advisor names.
    If you cannot find three advisors that the student is explicitly
    mentioning in acknowledgments, then use title page.
    Make sure to exclude the author's own name.

    If there are more than 3 advisors, then put 3 in the 'Advisors' list.
    Put the others in the 'Committee members' list.
```

```

If there are fewer than 3 advisors, then only take the ones you are sure
of.

Output the data in this exact format:
"advisors_GPT = ['Advisor1', 'Advisor2']".
All the names must be elements of one list.

Task 2:
Find any committee members mentioned in the text.
These should be different from the advisors. They must be named as
members of the committee.

Output the data in the format:
"committee_GPT = ['Committee member1', 'Committee member2']".
All the names must be elements of one list.

"""},
{"role": "user", "content": """
You have a dataframe named df with columns 'advisors_GPT', '
committee_GPT'.

Each cell contains a list of values.
I want you to use the previous ChatGPT output to overwrite this
dataframe.

Please provide a code that overwrites this dummy dataframe with the
output from the previous request.

Do not include any additional info in your output.
Do not import any packages.

Ideal example of the output format:
diss_df = pd.DataFrame(
    {'advisors_GPT': [['Heidi Williams', 'Amy Finkelstein',
'Joshua Angrist']],
    'committee_GPT': [['None']]}))
The output must start with: "diss_df ="
"""},
]

# Generate a response
response = openai.ChatCompletion.create(
    model = "gpt-4",
    messages=input,
    temperature=0.2)

output = response['choices'][0]['message']['content']

return output

```

## 2 Publications Data and Journal Lists

EconLit indexes nearly 2,000 journals, covering the entire spectrum of economics outlets as well as many from adjacent fields. Econlit also includes articles from collective volumes like the handbooks published by Elsevier and the NBER Macro Annual. To avoid overcounting publications by journal editors, we exclude forewords, editorial comments, and other types of editorial errata.

Rather than rely on the full list of journals indexed by Econlit, which changes considerably over time and contains many little-read and rarely-cited publications, we focus on two sets of journals. The first is based on the list generated for a study of the impact of economics scholarship (Angrist et al., 2020), referred to here as the "Deep Impact" (DI) journal list after

the paper’s title. For each discipline studied, Angrist et al. (2020) selects a ”trunk journal” (the *American Economic Review* for economics) and retains the fifty journals most cited by the trunk journal in any decade from 1970 to 2015 (non-economics discipline lists tend to be shorter than 50). The DI list used here includes EconLit journals found on the Angrist et al. (2020) discipline-specific lists for economics and related fields such as accounting, finance, management, marketing, multidisciplinary science, operations research, political science, sociology, and statistics. To this, we add a relatively new AEA journal not on the DI list (AEJ: Micro) and the relatively new Econometric Society journal, Quantitative Economics. The DI list contains 137 journals.

The second list consists of a set of ”Top 6” journals, matching that used in Angrist et al. (2020). This consists of the usual economics top 5 plus The Review of Economics and Statistics, which once had a similar standing as a general interest journal. We do not distinguish between the AEA Papers and Proceedings and the rest of the AER.

With a few exceptions, when looking for publications in a journal in Econlit the journal is identified by its ISSN. The exceptions are *IMF Staff Papers*, the *NBER Macroeconomics Annual*, and the *Journal of Economic and Social Measurement*, which are found by journal name. The DI list accounts for the vast majority of the citations made by papers published in the AER.

**Table B2:** Deep Impact Journal List

| Deep Impact                                           |                    |        |
|-------------------------------------------------------|--------------------|--------|
| Journal                                               | First Year Indexed | Papers |
| Accounting Review                                     | 1985               | 2123   |
| Aea Papers And Proceedings                            | 2018               | 776    |
| American Economic Journal: Applied Economics          | 2009               | 628    |
| American Economic Journal: Economic Policy            | 2009               | 678    |
| American Economic Journal: Macroeconomics             | 2009               | 540    |
| American Economic Journal: Microeconomics             | 2009               | 654    |
| American Economic Review                              | 1985               | 7099   |
| American Economic Review: Insights                    | 2019               | 154    |
| American Journal Of Agricultural Economics            | 1985               | 4441   |
| American Political Science Review                     | 1985               | 1679   |
| Annals Of The AAPSS                                   | 1998               | 1955   |
| Annual Review Of Financial Economics                  | 2009               | 74     |
| Brookings Papers On Economic Activity                 | 1985               | 1380   |
| Canadian Journal Of Economics                         | 1985               | 2375   |
| Carnegie-Rochester Conference Series On Public Policy | 1985               | 410    |
| Columbia Journal Of World Business                    | 1994               | 99     |
| Contemporary Accounting Research/Recherche Comptable  | 2003               | 1189   |
| Contemporaine                                         |                    |        |
| Demography                                            | 1985               | 2241   |
| Econometric Theory                                    | 1990               | 1474   |
| Econometrica                                          | 1985               | 2488   |
| Economic Development And Cultural Change              | 1985               | 1318   |
| Economic Inquiry                                      | 1985               | 2587   |
| Economic Journal                                      | 1985               | 3432   |
| Economic Record                                       | 1985               | 1335   |
| Economic Theory                                       | 1991               | 2611   |

| Deep Impact (continued)                           |                    |        |
|---------------------------------------------------|--------------------|--------|
| Journal                                           | First Year Indexed | Papers |
| Economica                                         | 1985               | 1389   |
| Economics Letters                                 | 1988               | 11136  |
| European Economic Review                          | 1985               | 4262   |
| European Journal Of Operational Research          | 2015               | 4274   |
| Experimental Economics                            | 1998               | 719    |
| Explorations In Economic History                  | 1985               | 945    |
| Financial Analysts Journal                        | 2012               | 299    |
| Financial Management                              | 1990               | 1020   |
| Games And Economic Behavior                       | 1989               | 3396   |
| Ilr Review                                        | 2015               | 361    |
| Industrial And Labor Relations Review             | 1985               | 1102   |
| Industrial Relations                              | 1985               | 1098   |
| Informa Journal On Applied Analytics              | 2017               | 178    |
| Interfaces                                        | 2012               | 212    |
| International Economic Review                     | 1985               | 2079   |
| International Journal Of Production Economics     | 1994               | 7052   |
| International Monetary Fund Staff Papers          | 1985               | 437    |
| International Organization                        | 1985               | 971    |
| Journal Of Accounting And Economics               | 1985               | 1176   |
| Journal Of Accounting Research                    | 1985               | 1372   |
| Journal Of Banking And Finance                    | 1985               | 5743   |
| Journal Of Business                               | 1985               | 700    |
| Journal Of Business And Economic Statistics       | 1985               | 2134   |
| Journal Of Business Ethics                        | 2020               | 1104   |
| Journal Of Business Finance And Accounting        | 2005               | 957    |
| Journal Of Consumer Affairs                       | 1986               | 1003   |
| Journal Of Consumer Research                      | 1985               | 2133   |
| Journal Of Corporate Finance                      | 1994               | 2262   |
| Journal Of Development Economics                  | 1985               | 3059   |
| Journal Of Econometrics                           | 1985               | 4414   |
| Journal Of Economic And Social Measurement        | 1985               | 536    |
| Journal Of Economic Behavior And Organization     | 1985               | 5799   |
| Journal Of Economic Dynamics And Control          | 1985               | 3816   |
| Journal Of Economic Education                     | 1985               | 1430   |
| Journal Of Economic History                       | 1985               | 1390   |
| Journal Of Economic Literature                    | 1985               | 822    |
| Journal Of Economic Perspectives                  | 1987               | 1918   |
| Journal Of Economic Theory                        | 1985               | 4008   |
| Journal Of Economics And Business                 | 1985               | 1182   |
| Journal Of Economics And Management Strategy      | 1992               | 1032   |
| Journal Of Environmental Economics And Management | 1985               | 2141   |
| Journal Of Finance                                | 1985               | 3093   |
| Journal Of Financial And Quantitative Analysis    | 1985               | 1915   |
| Journal Of Financial Economics                    | 1985               | 3271   |
| Journal Of Financial Intermediation               | 1990               | 708    |
| Journal Of Financial Markets                      | 1998               | 665    |
| Journal Of Financial Research                     | 1985               | 1054   |

| Deep Impact (continued)                                                      |                    |        |
|------------------------------------------------------------------------------|--------------------|--------|
| Journal                                                                      | First Year Indexed | Papers |
| Journal Of Financial Services Research                                       | 1987               | 866    |
| Journal Of Futures Markets                                                   | 1985               | 1928   |
| Journal Of Health Economics                                                  | 1985               | 2303   |
| Journal Of Human Resources                                                   | 1985               | 1465   |
| Journal Of Industrial Economics                                              | 1985               | 1109   |
| Journal Of International Business Studies                                    | 1998               | 1484   |
| Journal Of International Economics                                           | 1985               | 2448   |
| Journal Of International Money And Finance                                   | 1985               | 2879   |
| Journal Of Labor Economics                                                   | 1985               | 1274   |
| Journal Of Law And Economics                                                 | 1985               | 1083   |
| Journal Of Law Economics And Organization                                    | 1985               | 934    |
| Journal Of Legal Studies                                                     | 1988               | 780    |
| Journal Of Marketing Research                                                | 2009               | 975    |
| Journal Of Mathematical Economics                                            | 1985               | 2226   |
| Journal Of Monetary Economics                                                | 1985               | 2690   |
| Journal Of Money Credit And Banking                                          | 1985               | 2649   |
| Journal Of Peace Research                                                    | 1993               | 1323   |
| Journal Of Political Economy                                                 | 1985               | 2097   |
| Journal Of Portfolio Management                                              | 1985               | 2013   |
| Journal Of Public Economics                                                  | 1985               | 3829   |
| Journal Of Risk And Insurance                                                | 1985               | 1375   |
| Journal Of Risk And Uncertainty                                              | 1988               | 912    |
| Journal Of The American Statistical Association                              | 1985               | 4118   |
| Journal Of The European Economic Association                                 | 2003               | 1240   |
| Journal Of The Royal Statistical Society: Series A                           | 1985               | 24     |
| Journal Of The Royal Statistical Society: Series A (Statistics In Society)   | 1988               | 1366   |
| Journal Of The Royal Statistical Society: Series B (Statistical Methodology) | 2016               | 410    |
| Journal Of Urban Economics                                                   | 1985               | 1926   |
| Kyklos                                                                       | 1985               | 1009   |
| Land Economics                                                               | 1985               | 1551   |
| Management Science                                                           | 2012               | 1999   |
| Manufacturing And Service Operations Management                              | 2009               | 563    |
| Marketing Science                                                            | 1985               | 1621   |
| Mathematical Finance                                                         | 1995               | 814    |
| Mathematical Methods Of Operations Research                                  | 1995               | 1165   |
| Monthly Labor Review                                                         | 1985               | 2279   |
| NBER Macroeconomics Annual                                                   | 1986               | 553    |
| National Tax Journal                                                         | 1985               | 1685   |
| Operations Research                                                          | 2009               | 1263   |
| Oxford Economic Papers                                                       | 1985               | 1495   |
| Oxford Economic Papers N. S.                                                 | 1986               | 214    |
| Population And Development Review                                            | 1985               | 1329   |
| Proceedings Of The National Academy Of Sciences                              | 1996               | 393    |
| Production And Operations Management                                         | 2014               | 1421   |
| Public Choice                                                                | 1985               | 3586   |

| Deep Impact (continued)                         |                    |        |
|-------------------------------------------------|--------------------|--------|
| Journal                                         | First Year Indexed | Papers |
| Quantitative Economics                          | 2010               | 391    |
| Quarterly Journal Of Economics                  | 1985               | 1715   |
| Quarterly Journal Of Political Science          | 2006               | 287    |
| Quarterly Review Of Economics And Business      | 1985               | 219    |
| Rand Journal Of Economics                       | 1985               | 1523   |
| Research Policy                                 | 1997               | 3196   |
| Review Of Accounting Studies                    | 1996               | 890    |
| Review Of Economic Dynamics                     | 1998               | 1161   |
| Review Of Economic Studies                      | 1985               | 1922   |
| Review Of Economics And Statistics              | 1985               | 3108   |
| Review Of Finance                               | 2004               | 780    |
| Review Of Financial Studies                     | 1989               | 2376   |
| Scandinavian Journal Of Economics               | 1985               | 1648   |
| Social Choice And Welfare                       | 1985               | 2086   |
| Social Science Quarterly                        | 1985               | 2832   |
| Southern Economic Journal                       | 1985               | 2533   |
| Transportation Research: Part B: Methodological | 1999               | 2310   |
| Urban Affairs Review                            | 2005               | 770    |
| World Development                               | 1985               | 6841   |

**Table B3:** Top-6 Journal List

| Top-6                              |                    |        |
|------------------------------------|--------------------|--------|
| Journal                            | First Year Indexed | Papers |
| Aea Papers And Proceedings         | 2018               | 776    |
| American Economic Review           | 1985               | 7099   |
| Econometrica                       | 1985               | 2488   |
| Journal Of Political Economy       | 1985               | 2097   |
| Quarterly Journal Of Economics     | 1985               | 1715   |
| Review Of Economic Studies         | 1985               | 1922   |
| Review Of Economics And Statistics | 1985               | 3108   |

## References

Angrist, J., Azoulay, P., Ellison, G., Hill, R., and Lu, S. F. (2020). Inside job or deep impact? extramural citations and the influence of economic scholarship. *Journal of Economic Literature*, 58(1):3–52.
